# Supplementary material for: Analogical Inference for Multi-Relational Embeddings
Source: arXiv:1705.02426 source file (2017-07-06)
Supplement: Supplementary file 1 [file Appendix.tex]

\section{Appendix}
Note that combining Lemma \ref{le:conjugate_eigen} and Theorem \ref{thm:commutativity} could not trivially give rise to Corollary \ref{coro:alternative} since the real orthogonal basis in \ref{thm:commutativity} does not correspond to the block diagonalization basis in \ref{le:conjugate_eigen}. We therefore give out the detailed proof of Corollary \ref{coro:alternative}. Namely, we want to prove that there exists a \textit{real} orthogonal matrix $Q_r$ that block-diagonalizes all the commuting normal family matrices.

The proof can be divided into two parts: 
\begin{itemize}
\item We first prove that there exists a unitary matrix $Q$ which could be used to diagonalize the commuting family, and such $Q$ has exactly conjugate columns if the corresponding diagonalized entries have conjugate eigen-values.
\item Next, based on such $Q$,  we try to construct a real orthogonal matrix $Q_r$ that complements the proof.
\end{itemize}
\begin{lemma}
		\label{le:conjugate_eigen}
	For real normal matrices $A_1,A_2,\dots$ that form a commuting family, there exists a unitary $Q$ that diagonalizes all matrices and $\forall A_i$, if a column $q\in Q$ is the eigen-vector corresponding to some complex eigen-value $\lambda\not\in \mathbb{R}$, its conjugate $\bar{q}$ is also one column of $Q$.
\end{lemma}
\begin{proof}
	First, by Theorem \ref{thm:commutativity}, we see that there exists a unitary $Q_0$ that diagonalizes all matrices. We then show how to construct such $Q$ based on $Q_0$. This purpose can be done by an iterative process.
	
	Consider $A_1$. For any complex (non-real) eigen-value $\lambda$ of $A_1$, suppose its corresponding eigen-vectors are columns $q_1,\dots,q_k\in Q$. i.e.
	\begin{align}
	A_1q_i=\lambda q_i, \forall i\in \{1,\dots,k\}
	\end{align}
	As $A_1$ is real, by taking the conjugate of the above equation, we notice that
	\begin{align}
	\label{eq:conjugate_eigen}
	A_1\bar{q_i}=\bar{\lambda} \bar{q_i}, \forall i\in \{1,\dots,k\}
	\end{align}
	This shows $\bar{\lambda}$ is also an eigen-value of $A_1$, and the corresponding geometric multiplicity under $\bar{\lambda}$ should be at least $k$. By symmetry, we see that $\lambda$ should also have a larger dimension of eigen-space than $\bar{\lambda}$. This indicates that $\bar{\lambda}$ should have exactly an eigen-space of dimension $k$ (geometric multiplicity).
	
	Without loss of generality, suppose the eigen-vectors of $\bar{\lambda}$ are exactly columns $q_{k+1},\dots,q_{2k}$. We prove that by replacing them with $\bar{q_1},\dots, \bar{q_k}$, the new matrix $Q_1$ could still diagonalize all matrices $A_1,A_2\dots$.  In fact, since $q_1$ is an eigen-vector of $A_1,A_2\dots$, $\bar{q_1}$ should also be an eigen-vector of $A_1,A_2,\dots$ by similar argument in Equation \ref{eq:conjugate_eigen}, which suggests the diagonalization.
	
	Besides, we see that $Q_1$ is still a unitary matrix. Actually, by the equivalence of eigen-space under $\bar{\lambda}$: $\text{span}(q_{k+1},\dots,q_{2k})=\text{span}(\bar{q_1},\dots, \bar{q_k})$, there exists a unitary matrix $U_0$ such that $[\bar{q_1},\dots, \bar{q_k}]=[q_{k+1},\dots,q_{2k}]U_0$. One can find $Q_1=UQ_0$ where $U$ is a block-diagonal matrix that has $1$ on the diagonal entries except a sub-block $U_1$ at the left-most corner. This means $U$ is still a unitary matrix, thus showing $Q_1$, the product of two unitary matrices, keeps unitarity.
	
	Therefore, by one step of such modification, we find a new unitary  $Q_1$ that diagonalize all $A_1,A_2\dots$. By repeating such processes, we can finally get the $Q$ that have columns all conjugate once the eigen-values are conjugate. One point to note is that we only prove the columns are conjugate once eigen-values in $A_1$ are conjugate. We could apply such modification on $A_2,A_3,\dots$ iteratively without breaking established conjugate pairs, and make the conjugate column condition hold for any $A_i$. ({\color{red} may extend}.)  
	
	Namely, for the final $Q$, if $q\in Q$ corresponds to some complex $\lambda$ of $ A_i$, we could also have $\bar{q} \in Q$ which belongs to eigen-value $\bar{\lambda}$ of $A_i$. Besides, the corresponding eigen-values are also conjugate to each other for any $A_j\neq A_i$,
	 as $ A_jq=\lambda_j q\iff A_j\bar{q}=\bar{\lambda}_j \bar{q}$. 
	% Suppose the diagonalized matrices (after $Q_1$) to be $\Lambda_1, \Lambda_2,\dots$.	
	% Namely, if $A_2$ were to replace some $q_{k+1},\dots, q_{2k}$ with $q_1,\dots, q_k$
\end{proof}
\subsection{Complete Proof of Corollary \ref{coro:alternative}}
\begin{proof}[Complete Proof]
	By Lemma \ref{le:conjugate_eigen}, we can find such $Q$, s.t. as long as there's some complex eigen-value $\lambda$ of $A_i$ and its eigen-vector $q$ in $Q$, the conjugate $\bar{q}$ is also in $Q$. And the eigen-values are also conjugate for any $A_j$.
	
	Denote the conjugate pair to be $q=a+bi$ and $\bar{q}=a-bi$ where $a,b\in \mathbb{R}^{n}$. And suppose for any $A_i$, the corresponding eigen-values are $\alpha+\beta i$ and $\alpha-\beta i$ where $\alpha,\beta \in \mathbb{R}$. We know that
	\begin{align}
	&A_i(a+bi)=(\alpha+\beta i)(a+bi)\\
	\iff &A_i a=\alpha a-\beta b\\
	&A_i b=\beta a+b\alpha\\
	\label{eq:unnorm_eigen}
	\iff &A_i[a, b]=[a,b]\begin{bmatrix}
	\alpha, &-\beta\\	
	\beta, &\alpha
	\end{bmatrix}
	\end{align}
	We prove that by replacing $q,\bar{q}$ with $\frac{a}{\|a\|}$, $\frac{b}{\|b\|}$ we could obtain $\begin{bmatrix}
	\alpha, &-\beta\\	
	\beta, &\alpha
	\end{bmatrix}$ blocks.
	
	Actually, as $q\perp \bar{q}$, we know that
	\begin{align}
		&\langle q, \bar{q}\rangle=0\\
		\iff&(a^{\top}-b^{\top}i)(a-bi)=0\\
		\iff&a^{\top}a=b^{\top}b\\
				&a^{\top}b=0
	\end{align}
	Besides, as $\langle q, q\rangle=1$, we see that $a^{\top}a+b^{\top}b=1$. Thus, $\|a\|^2=\|b\|^2=1/2$. 	Therefore, Equation \ref{eq:unnorm_eigen} leads to
	\begin{align}
	A_i[a/\|a\|, b/\|b\|]=	A_i[\sqrt{2}a,\sqrt{2} b]=[a/\|a\|,b/\|b\|]\begin{bmatrix}
	\alpha, &-\beta\\	
	\beta, &\alpha
	\end{bmatrix}
	\end{align}
	 Also, $a,b$ are perpendicular to other columns of $Q$ since both the real part and the imaginary part have to be perpendicular to $Q$ due to unitarity. Thus, this replacement keeps both orthogonality and gives rise to $2\times 2$ sub-blocks.
	 
	 By repetitive processes, we could replace all such conjugate pairs with real orthogonal bases. Thus we only need to change the remaining eigen-vectors corresponding to real eigen-values under all $A_1,A_2,\dots$. In fact, we could directly replace them with the real/imaginary parts to keep the orthogonality. Actually, if $q=a+bi\in \mathbb{C}^n,\lambda \in \mathbb{R}$ w.r.t. $A_i$, we could find
	 \begin{align}
	 	&A_i (a+bi)=\lambda (a+bi)\\
	 	\iff &A_ia=\lambda a\\
	 	&A_ib=\lambda b
	 \end{align}
	 This suggests that both $a$ and $b$ are eigen-vectors of $A_i$. As $q=a+bi$ is the column of unitary $Q$, we know that $a,b$ could not both be linearly dependent on all the other columns. Then we could simply replace $q$ with the (normalized) linearly independent one and still keeps the orthogonality and do not change the $1\times 1$ sub-blocks of the diagonalized matrices.
	 
	 Combining both procedures dealing with complex and real eigen-values, we could finish up the construction of $Q_r$ and get only $1\times 1$ and $2\times 2$ sub-blocks for the final block-diagonal matrices.
%	We replace these two columns with $\{u,v\}$, an orthogonal basis of $\text{span}(a,b)$. Since $a,b$ are independent, there exists a real invertible matrix $C\in \mathbb{R}^{2\times 2}$ with
%	\begin{align}
%		[u,v]=[a, b]C
%	\end{align}
%	Therefore, 
%	\begin{align}
%		A_i[u,v]=A_i[a, b]C=[a,b]\begin{bmatrix}
%		\alpha, &-\beta\\	
%		\beta, &\alpha
%		\end{bmatrix}C=[u,v]C^{-1}\begin{bmatrix}
%		\alpha, &-\beta\\	
%		\beta, &\alpha
%		\end{bmatrix}C\\
%	\end{align}
%	If λ is a real eigenvalue, we can assume without loss of generality that the corresponding eigenvector is real.
\end{proof}
